# Supplementary material for: An Examination of Grouping and Spatial Organization Tasks for High-Dimensional Data Exploration
Source: arXiv:2008.09233 source file (2020-08-20)
Supplement: Supplementary file 1 [file Supplemental_Material.pdf]

# Supplemental Material for “An Examination of Grouping and Spatial Organization Tasks for High-Dimensional Data Exploration”

Study Pre-Survey ....................................................1
Study Post-Survey...................................................2
Informed Consent Form..........................................3
Recruitment Email ..................................................5
All Notecards ..........................................................6
Dataset.....................................................................7

## Study Pre-Survey

1. Rate your familiarity with dimensionality reduction algorithms.
   a. Never heard of them
   b. Have heard about them, but have never used them
   c. Have used them, but do not fully understand them
   d. I am an expert

2. Rate your familiarity with clustering algorithms.
   a. Never heard of them
   b. Have heard about them, but have never used them
   c. Have used them, but do not fully understand them
   d. I am an expert

3. Is it possible to visualize (e.g., via a graph) a dataset with more than 3 dimensions?
   a. Yes
   b. No
   c. I’m not sure

4. Briefly describe your experience with exploratory data analysis and/or data science.
   <free response>

<u>Study Post-Survey</u>

1. What was your high-level strategy?  How did you think you approached the task?
   <free response>

2. What was the easiest part of the tasks that you performed?
   <free response>

3. What was the most difficult part of the tasks that you performed?
   <free response>

4. Did you find the grouping or the spatialization operations to be more useful?  Why?
   <free response>

5. Did you find the grouping or the spatialization operations to be more meaningful?  Why?
   <free response>

6. Do you think you performed more grouping or spatialization operations?
   <free response>

Informed Consent Document

**Informed Consent for Participant of Investigative Project**
Virginia Polytechnic Institute and State University

**Title of Project:** Interactive Visual Data Analysis
**Principal Investigators:** Dr. Chris North, John Wenskovitch

1. **Purpose:** You are invited to participate in a study examining how humans physically analyze and explore data, with the goal of understanding the aspects of human cognition that underlie this process.

2. **Procedures:** (1) You will be asked to complete a demographic questionnaire. (2) You will be asked to analyze and physically organize some data, using interactive software or physical papers. This organizing will occur incrementally, and you will be asked to verbalize your actions to understand your thought process. After you reach a satisfactory conclusion, you will be asked to describe your analysis result more generally. (3) You will then be asked to continue your analysis, based on updated information about the data. The incremental procedure from the previous step will be repeated. (4) You will be asked to participate in an exit survey. Phases (2) and (3) will include video recordings maintained in a password-protected folder on a researcher's computer.

3. **Risks:** There is minimal risk involved with this study. The experiment involves performing everyday office work with a desk or computer. You will be organizing a collection of data using software or papers, which includes a slight risk of paper cuts. Mild mental fatigue is also possible, due to the cognitive requirements of the organizational tasks. Visual or interactive fatigue is also possible while using computer software. You will be able to ask questions during your session, and additional time to complete the task can be arranged if you should feel overly exerted. If you experience any discomforts, please feel free to stop and inform the experimenter.

4. **Benefits of this Project:** Your participation in this study will provide information that may be used to inform the design of support tools and applications for analyzing and comprehending complex data. The results of this study will be published and included in a PhD dissertation.

5. **Compensation:** You will be entered into a drawing for one of five $20 electronic gift cards.

6. **Extent of Anonymity and Confidentiality:** The results of this study will be kept strictly confidential. Your written consent is required for the researchers to release any data identified with you as an individual to anyone other than personnel working on the project. Only unique subject numbers will be used in analysis and reports.

7. **Approval of Research:** This research has been submitted to the Institutional Review Board for projects involving human subjects at Virginia Polytechnic Institute and State University.

8. **Subject's Responsibilities and Permission:** I hereby acknowledge the above and give my voluntary consent for participation in this project. If I participate, I may withdraw at any time without penalty. I agree to abide by the rules of this project.

9. **Who can I talk to?** If you have questions, concerns, or complaints, or think the research has hurt you, talk to the research team.


| | | |
|---|---|---|
| **Investigator:** | Chris North<br>Professor<br>Computer Science<br>Virginia Tech | Email: north@vt.edu<br>Phone: +1 (540) 231-2458 |


This research has been reviewed by the Virginia Tech Institutional Review Board (IRB). You may communicate with them at 540-231-3732 or irb@vt.edu if:

- You have questions about your rights as a research subject
- Your questions, concerns, or complaints are not being answered by the research team
- You cannot reach the research team
- You want to talk to someone besides the research team to provide feedback about this research

**Name:** ________________________________ **Date:** ____________________

**Signature:** ________________________________

## Recruitment Email

**Subject:** Call for Participation: Cognitive User Study

You are invited to participate in a study about the organization process of human analysts to explore a numerical data set.

**Purpose:** Our overall goal in this study is to investigate the cognitive processes that underlie the specialization and grouping of objects represented by numerical data.

**Requirements:** Age 18+

**Experiment Details:** We anticipate that completion of this study will require about one hour.

1. You will be asked to fill out a short questionnaire. (estimated 5 minutes)
2. You will be asked to physically structure one dataset, consisting of numerical values written on index cards, on a tabletop. This structuring will occur incrementally, one card at a time, with questions after each interaction to understand your thought process. After you reach a satisfactory layout, you will be asked to describe your structure more generally. (estimated 20 minutes)
3. You will then be asked to update your layout, based on updated information regarding which aspects of the data should be prioritized in the layout. The incremental procedure from the previous step will be repeated. (estimated 20 minutes)
4. You will be asked to participate in an exit survey. (estimated 5 minutes)

Participation is confidential and completely voluntary. This study is being conducted for data collection purposes, intended for inclusion in a PhD dissertation and as an eventual publication. As a reward for completing this study, you will be entered into a drawing for one of two $20 gift cards.

If interested, please email John Wenskovitch at jw87@vt.edu.

Full Collection of Notecards

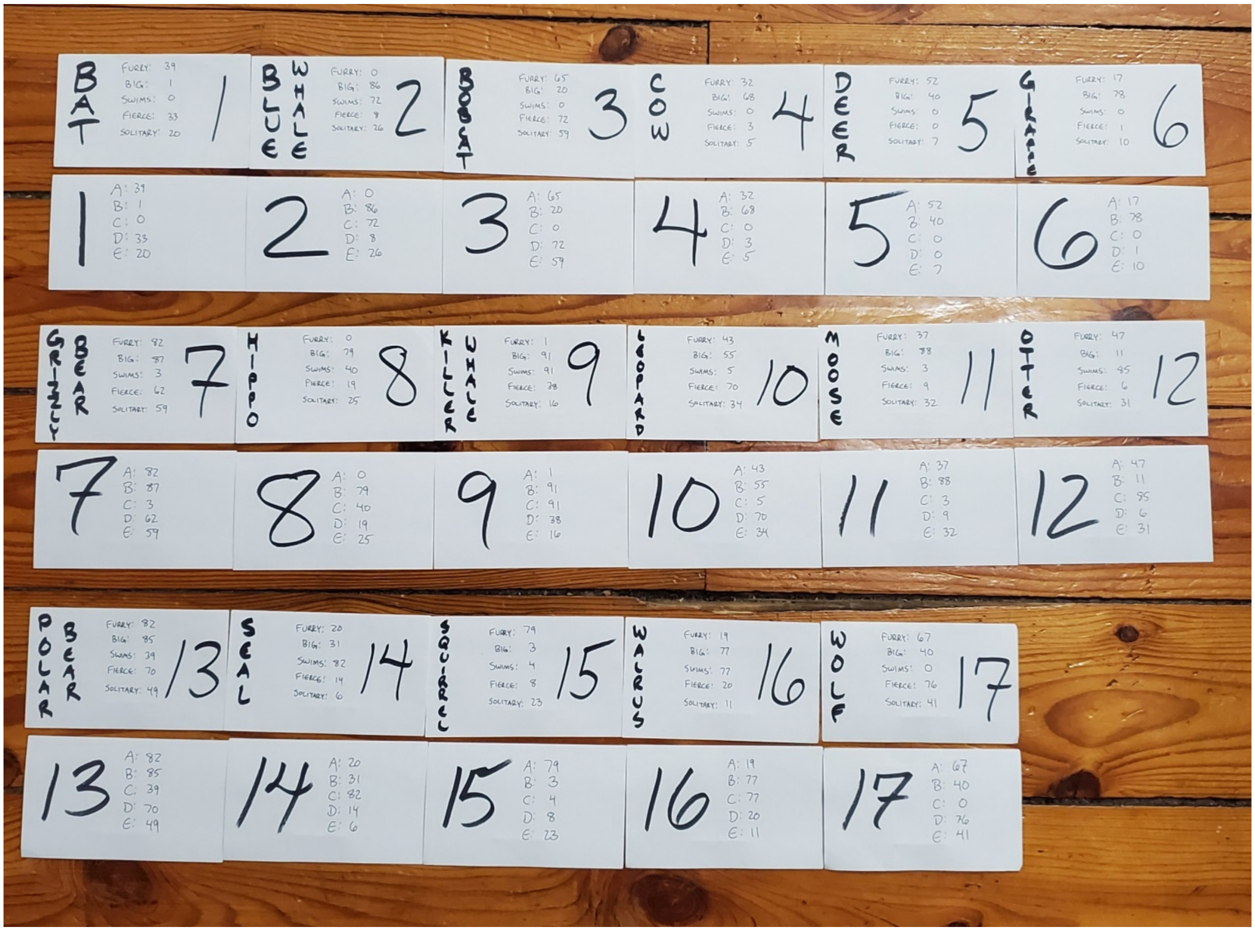

Dataset

| Animal | Furry | Big | Swims | Fierce | Solitary |
|---:|---|---|---|---|---|
| **Bat** | 39 | 1 | 0 | 33 | 20 |
| **Blue Whale** | 0 | 87 | 72 | 8 | 26 |
| **Bobcat** | 65 | 20 | 0 | 72 | 59 |
| **Cow** | 32 | 68 | 0 | 3 | 5 |
| **Deer** | 52 | 40 | 0 | 0 | 7 |
| **Giraffe** | 17 | 78 | 0 | 1 | 10 |
| **Grizzly Bear** | 82 | 87 | 3 | 62 | 59 |
| **Hippopotamus** | 0 | 79 | 40 | 19 | 25 |
| **Killer Whale** | 1 | 91 | 91 | 38 | 16 |
| **Leopard** | 43 | 55 | 5 | 70 | 34 |
| **Moose** | 37 | 88 | 3 | 9 | 32 |
| **Otter** | 47 | 11 | 85 | 5 | 31 |
| **Polar Bear** | 82 | 85 | 39 | 70 | 49 |
| **Seal** | 20 | 31 | 82 | 14 | 6 |
| **Squirrel** | 79 | 3 | 4 | 8 | 23 |
| **Walrus** | 19 | 76 | 77 | 20 | 11 |
| **Wolf** | 67 | 40 | 0 | 76 | 41 |
